# Supplementary material for: Skill-Critic: Refining Learned Skills for Hierarchical Reinforcement Learning
Source: arXiv:2306.08388 source file (2024-07-12)
Supplement: Supplementary file 2 [file appendix_arxiv.tex]

% \appendix
\section*{Appendix}
\setcounter{section}{0}
\section{Implementation and Experimental Details} 
\subsection{Implementation: Offline Skill Prior and Embedding Pre-Training} \label{Subsec:learn_skill}
 In Section \ref{Sec:skillprior}, we pre-train a skill embedding space and skill prior from offline data to accelerate downstream RL. Pre-training consists of training a Variational Auto-Encoder \cite{kingma2013auto} as in previous skill-transfer RL \cite{nair2020awac, pertsch2021guided}. 
 A skill, $a^i_{0:H-1}$, is a sequence of actions $a^i_{0:H-1} = \{a^i_0, ..., a_{H-1}^i\}$ with a fixed horizon $H$, and  the state-sequence associated with these actions is $s^i_{0:H-1}=\{s_0, s_1^i ..., s_{H}^i\}$ starting from initial state $s_0$. 
We use a state-dependent skill decoder $g_{\psi_z}(a|s,z)$  \cite{pertsch2021guided} which shows improved performance over a state-agnostic decoder, i.e. $g(a_{0:H-1}|z)$ \cite{pertsch2021accelerating}.

\textbf{VAE \newtextsmall{and Skill Prior} Training. }We formulate the skill inference network (encoder) as $q_\zeta(z|a_{0:H-1}, s_{0:H-1})$ and the closed-loop skill policy network (decoder) as
$g_{\psi_a}(a|s,z)$, as deep neural networks parameterized by $\zeta$ and $\psi_a$. 
We randomly sample $H$-step trajectories, $(a_{0:H-1},s_{0:H-1})$, from the full demonstration trajectories, and train the latent skill embedding  using variational inference:
\begin{equation} \label{Eqn:VAE}
\max _{\psi_a, \zeta, \psi_z} \mathbb{E}_q\biggl[
\underbrace{\prod_{k=0}^{H-1} \log g_{\psi_a}\left(a_k | s_k,z_k \right)}_{\text{reconstruction}}
-\beta_{\mathrm{VAE}}
\underbrace{\biggl(\log q_\zeta\left(z_k | a_{0:H-1}, s_{0:H-1}\right)-\log p(z_k)\biggr)}_{\text{regularization}}+\mathcal{L}_{_{\psi_z}}\biggr].
\end{equation}
The prior $p(z)$ is a unit Gaussian $\mathcal{N}(0,I)$ and $\beta_{\mathrm{VAE}}$ is a regularization factor.  \begin{newtext}The skill encoder, $q_\zeta\left(z |s_{0:H-1},a_{0:H-1}\right)$, parameterizes the Gaussian distribution $\mathcal{N}\left(\mu_z, \sigma_z \right)$, which represents the posterior distribution of the skill, $z$, in the embedding space $\mathcal{Z}$, given the sequences of states, $s_{0:H-1}$, and actions, $a_{0:H-1}$. \end{newtext}
In practice, the reconstruction term in Eqn.~\eqref{Eqn:VAE} is a negative log-likelihood (NLL) loss between two deterministic sequences, which can be simplified as mean square error (MSE) \newtextsmall{as shown} in Eqn.~\eqref{Eqn: loss_skill}.

The skill-prior loss, $\mathcal{L}_{p_{\psi_z}}$, is introduced to the VAE train a skill prior distribution from the skill encoder \cite{pertsch2021accelerating, pertsch2021guided}. \begin{newtext}
We  build a skill-prior model, $p_{\psi_z}(z|s_0)$, with network parameters $\psi_z$. The skill prior imitates the skill posterior $q_\zeta$ by minimizing the reverse Kullback-Leibler divergence (KL divergence):\end{newtext}
\begin{equation} \label{Eqn:prior}
\min _{\psi_z} \mathbb{E}_{(s_t \sim D} \left[ D_{K L}\left(q_\zeta\left(z | a_{0:H-1}, s_{0:H-1}\right) \| p_{\psi_z}\left(z_t | s_t\right)\right) \right].
\end{equation}
%commment
  \newtextsmall{The skill prior, $p_\psi\left(z | s\right)$,} parameterizes the Gaussian distribution\newtextsmall{ $\mathcal{N}\left(\mu_p, \sigma_p \right)$, which is the prior }distribution of the skill, $z$, given the \newtextsmall{state $s$. }

  \begin{newtext}
  Thus to train the VAE and skill prior, we use the same objective function as in SPiRL with unit-variance Gaussian output distribution \cite{nair2020awac}, and Eqn. \eqref{Eqn:VAE} can be written as\end{newtext}
\begin{equation} \label{Eqn: loss_skill}
\mathcal{L}=\sum_{k=0}^{H-1} \underbrace{\left\|a_{k}-\hat{a}_k\right\|^2}_{\text{reconstruction}}
+\beta_{\textrm{VAE}} \underbrace{D_{K L}\left(\mathcal{N}\left(\mu_z, \sigma_z\right) \| \mathcal{N}(0, I)\right) }_{\text{regularization}} +
\underbrace{ D_{K L}\left(\mathcal{N}\left(\lfloor \mu_z \rfloor, \lfloor \sigma_z \rfloor \right) \| \mathcal{N}\left(\mu_p, \sigma_p\right)\right),}_{\text{prior training}}
\end{equation}
\begin{newtext}where $\hat{a}_k$ is the action predicted by the decoder network, $\hat{a}_k := g_{\psi_a}(a_k|s_k,z_k)$.
Here $\lfloor \cdot \rfloor$ denotes the gradient flow of these variables is stopped during training.\end{newtext}

 For the encoder, the state sequence $s_{0:H-1}$ is not augmented with the time index, $k$, since information is identical for all state sequences. The skill decoder, $g_{\psi_a}\left(a | s, z\right)$, employs a time-augmented state, $s$, to output the decoded action, $a$, given the skill, $z$, at each time step. Namely, the state, $s$, is augmented with a one-hot encoding of the time index since the start of the current skill, $k\doteq (t \mod H)$ for the decoder. 

\textbf{Pre-Training Details and Summary.}
We use the same network structure as SKilD~\cite{pertsch2021guided}, except for the decoder policy. The encoder is a 1-layer LSTM with 128 hidden units.  The skill prior is a 5-layer MLP with 128 hidden units per layer. We use a horizon $H=10$ and 10-dimensional skill representations, $z\in \mathcal{Z}$.  We tune the regularization weight $\beta_{\textrm{VAE}}$, finding the best performance at 1e-2 for the maze and 5e-2 for the racing environment. All networks use batch normalization after every layer and leaky ReLU action functions.

The decoder is a 3-layer MLP with 128 hidden units per layer. Unlike SKilD, to help with downstream learning, for the skill decoder only, we extend the state with a one-hot variable $k_t=(t\mod H)$ indicating the time index. Furthermore, the output layer of the decoder network outputs both $\mu_{\hat{a}}$ and $\sigma_0$; however, only $\mu_{\hat{a}}$ is trained in Eqn. \eqref{Eqn: loss_skill} and  $\sigma_0$ is a dummy value that is never used. This method ensures the decoder can initialize the LL policy, which outputs both mean and standard deviation. A procedure for introducing a low-level decoder variance, $\sigma_{\hat{a}}$, as a hyperparameter is used to regulate the LL policy as described in the following Appendix.

The outputs of this stage are the encoder and decoder mapping the skill embedding space, $\mathcal{Z}$ and the skill prior, $p_{\psi_z}(z|s)$, that characterizes a prior probability for the skill $z$ with respect to the state $s$. The skill encoder, $q_\zeta(z|s_{0:H-1},a_{0:H-1})$ maps state-action sequences into the skill space $\mathcal{Z}$. The skill policy decoder, $g_{\psi_a}(a|s,z)$, maps the state and active skill to the action. 

\subsection{Implementation Details: Downstream RL} \label{Appendix: downstream RL}

\paragraph{Variance of the Action Prior.} 
In the Skill-Critic algorithm, the HL and LL policies are meant to be initialized and regularized by the skill-prior and decoder networks, respectively. During downstream RL, continuous action exploration is often achieved using probabilistic policies, including in SAC \cite{haarnoja2018soft} and the HL policy update in SPiRL \cite{pertsch2021accelerating}. During VAE pre-training, both $\mu_{p}$ and $\sigma_p$ are trained as outputs of the skill prior, $p_{\psi_z}$, and the skill-prior network can be directly used to initialize the HL policy network, $\pi_{\theta_z}$. However, the VAE pre-training of the decoder network only trains the mean action of the decoder, $\mu_{\hat{a}}=g_{\psi_a}(a|s,z)$ \cite{pertsch2021accelerating}. Therefore, to promote exploration, it is necessary to include a non-zero LL variance as a prior distribution for the LL policy. 

The decoder parameters, $\psi_a$, are used to initialize the LL policy $\pi_{\theta_a}$, which is made possible since the decoder outputs $(\mu_{\hat{a}}, \sigma_0)$, where $\sigma_0$ is an unused dummy variable that serves as a placeholder to ensure the LL policy network and the decoder network architecture are identical.  Only the output $\mu_{\hat{a}}$ of the decoder is trained by the VAE, and $\sigma_0$ is never used.

We manually set the value of the decoder variance, $\sigma_{\hat{a}}$, and only the output corresponding to $\mu_{\hat{a}}$ from the decoder network $g_{\psi_a}$ is used during regularization. The decoder variance, $\sigma_{\hat{a}}$, is a hyperparameter that balances skill exploration and exploitation in the downstream LL policy \cite{levine2018reinforcement}. We define the \textbf{\textit{action prior}} distribution as a Gaussian distribution, i.e., $p_{\bar{\psi}_a}(a|s,z)=\mathcal{N}(\mu_{\hat{a}}, \sigma_{\hat{a}})$, where $\mu_{\hat{a}}$ is the output of the policy decoder $g_{\psi_a}$. In a slight abuse of notation, we denote the action prior as parameterized by $\bar{\psi}_a\doteq [\psi_a, \sigma_{a}]$. 

During downstream training, the LL policy network, $\pi_{\theta_a}$ outputs the values $\mu_{\pi_a}$ and $\sigma_{\pi_a}$. These values parameterize a Gaussian distribution for action selection,  $\mathcal{N}(\mu_{\pi_a}, \sigma_{\pi_a} +\sigma_{\hat{a}})$, where decoder variance $\sigma_{\hat{a}}$ is added to LL policy variance $\sigma_{\pi_a}$ to bias the initial value. Thus, during rollouts, actions are selected from the policy via $a\sim \mathcal{N}(\mu_{\pi_a}, \sigma_{\pi_a} +\sigma_{\hat{a}})$, where $\mu_{\pi_a}$ and $\sigma_{\pi_a}$ are the outputs of the network $\pi_{\theta_a}$ and $\sigma_{\hat{a}}$ is the fixed-value hyperparameter.  We denote the LL policy  regularization by
\begin{equation} \label{Eqn: DKL_LL}
    D_{K L}  \left(\pi_{\theta_a}\left(a \mid s, z\right) \|  p_{\bar{\psi}_a}\left(a \mid s, z\right)\right)  \doteq D_{K L}\left( \mathcal{N}( \mu_{\pi_a}, \sigma_{\pi_a} +\sigma_{\hat{a}}) \| \mathcal{N}(\mu_{\hat{a}} ,\sigma_{\hat{a}}) \right).
\end{equation}
% We note the similarity to the HL update policy regularization. As shown in SPiRL \cite{pertsch2021accelerating}, the 
This procedure allows us to ensure the action prior has a non-zero variance. This is important since policy variance plays a pivotal role in balancing action exploration and exploitation \cite{levine2018reinforcement}. We perform an ablation study on the parameter $\sigma_{\hat{a}}$ in Appendix \ref{Appendix: Ablation}. 

\paragraph{HL SPiRL Warm-start in Maze}
\begin{wrapfigure}{r}{0.5\textwidth}
    \centering
    \vspace{-3mm}
    \includegraphics[width=0.5\textwidth]{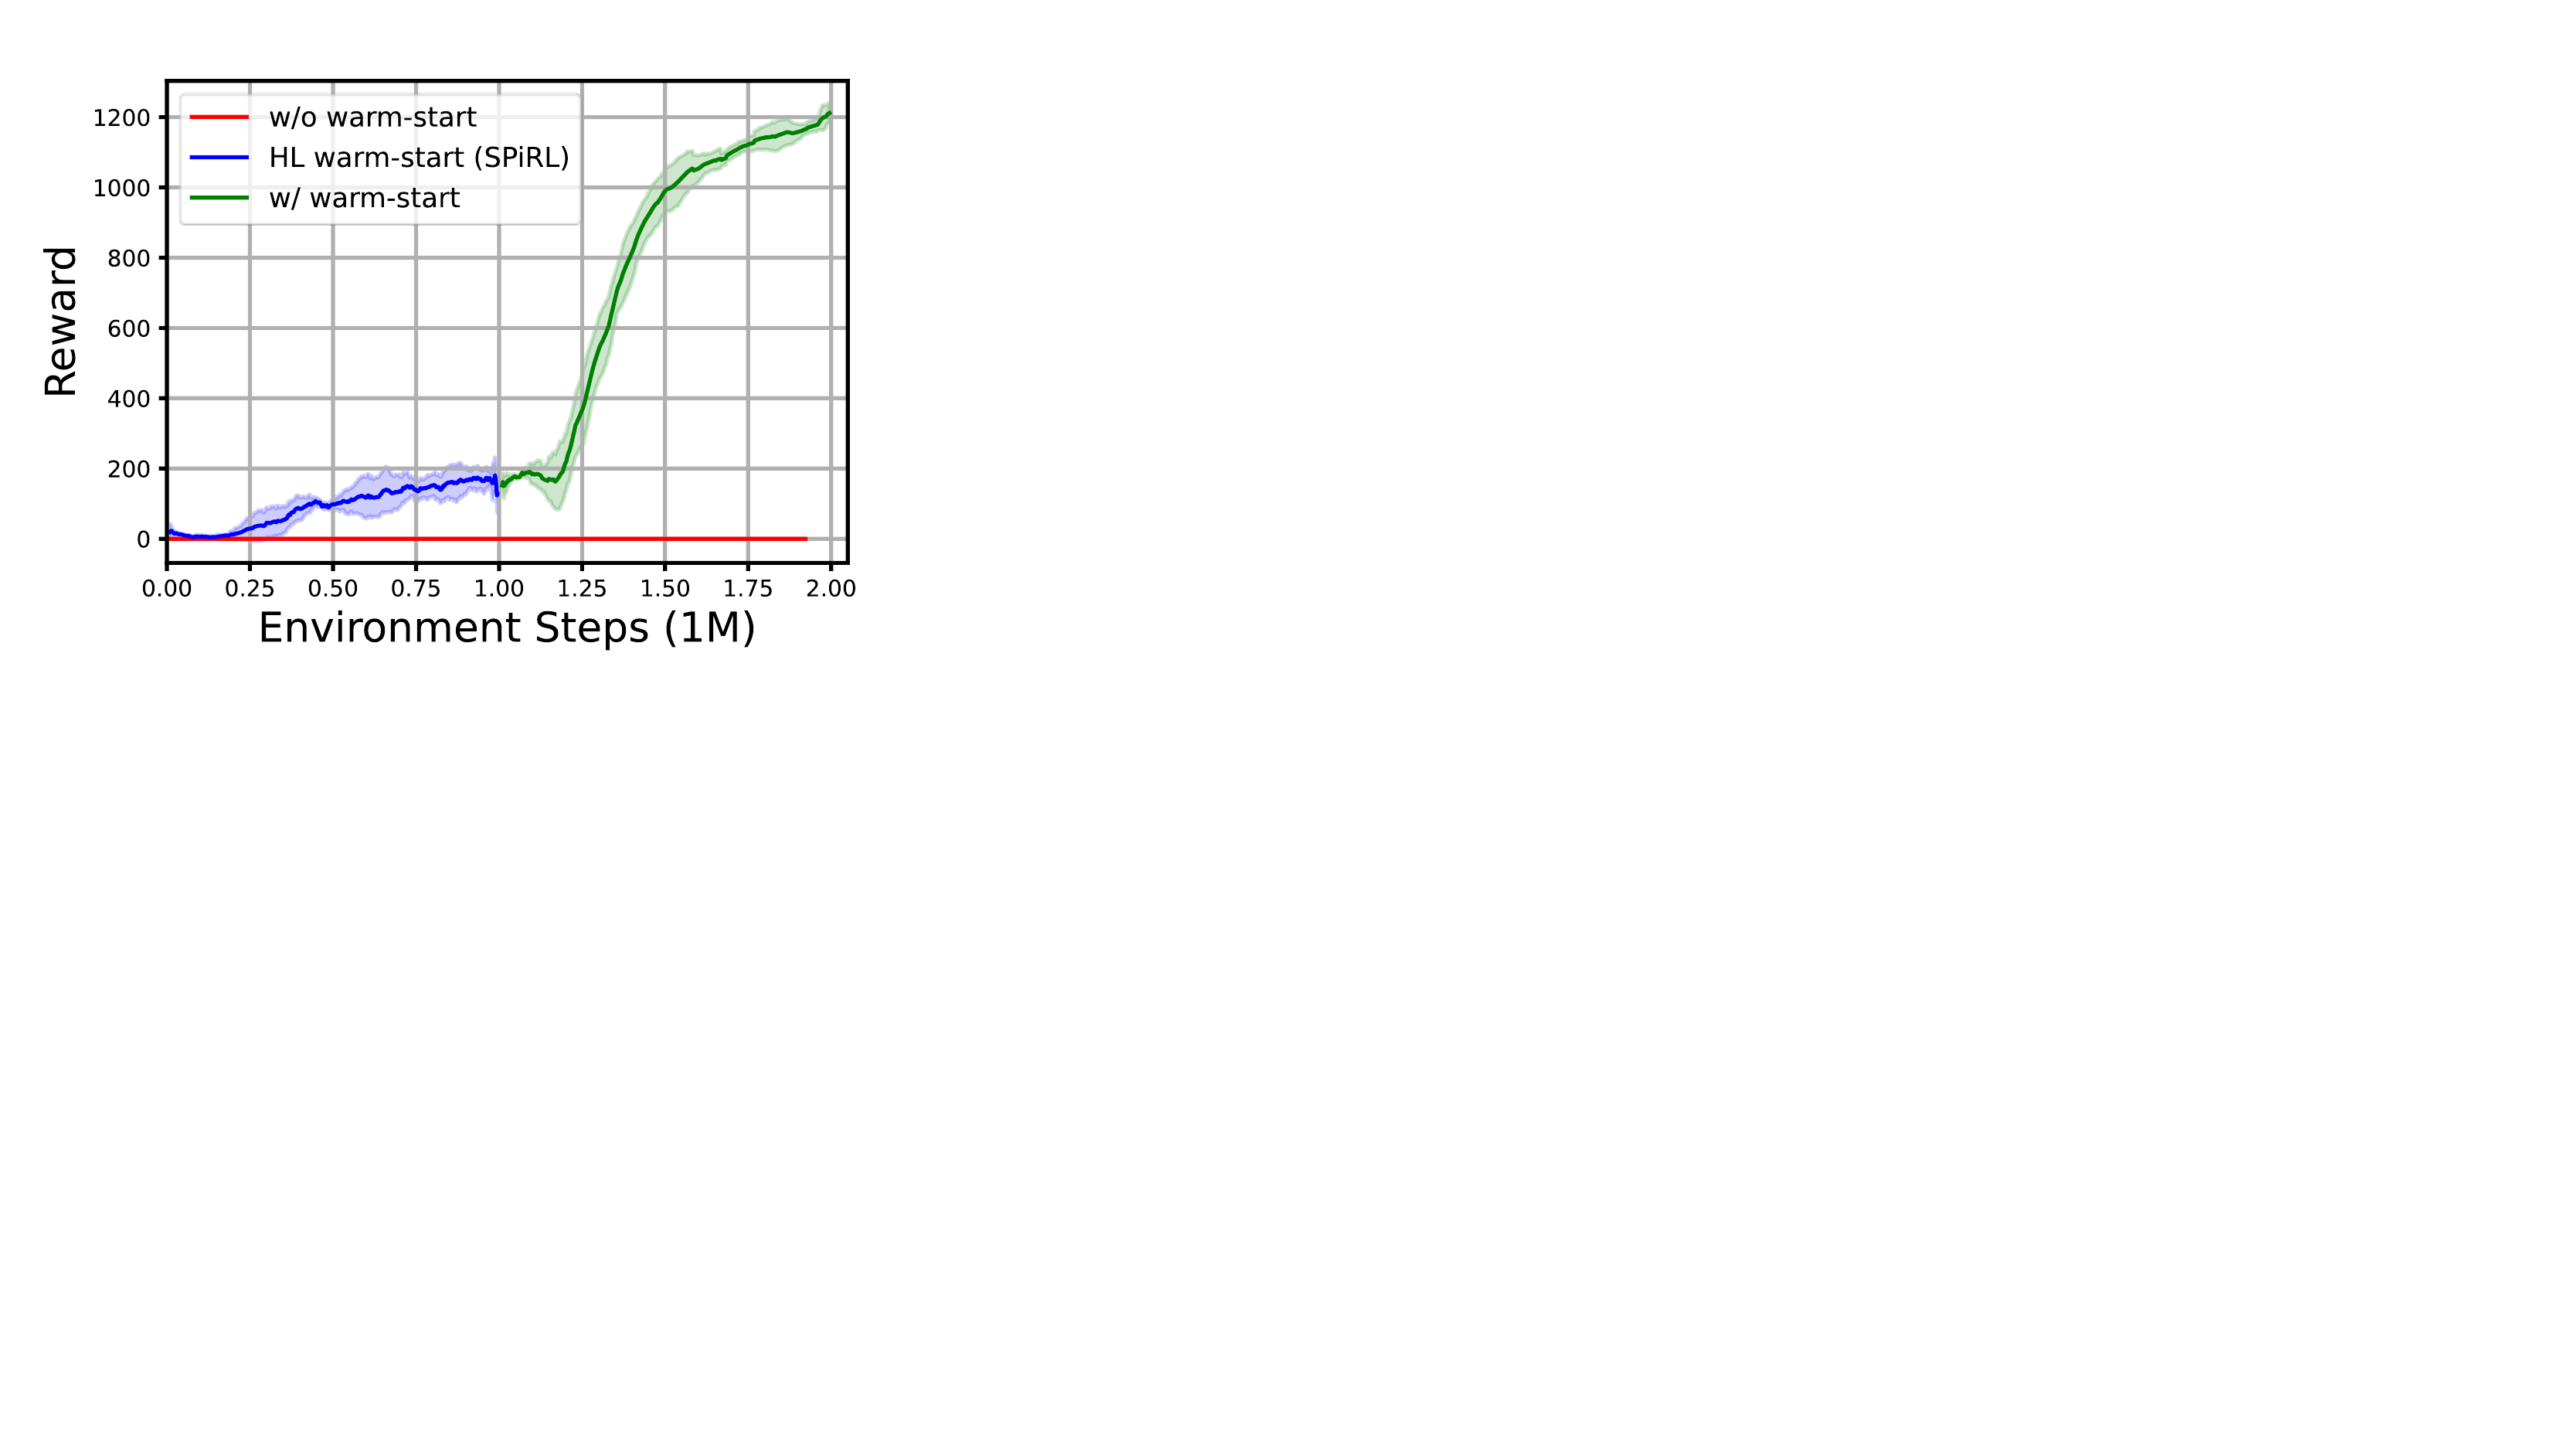}
    \caption{Skill-Critic training in maze navigation. We implement training without(w/o) warm-start, and with(w/) HL warm-start for 1 million steps.}
    \vspace{-2mm}
    \label{Fig: warm-start}
\end{wrapfigure}

When implementing the Skill-Critic algorithm in the maze environment, we warms-tart the HL policy, $\pi_z$, and Q-value, $Q^z$, using the SPiRL algorithm. 
Specifically, we train the HL policy alone with a stationary LL policy (removing line 11 in Algorithm~\ref{Alg:skill-critic-summary}) for 1 million steps, at which point a reasonable HL policy is found. This initial training step is exactly the problem in SPiRL, and it occurs after initializing the HL and LL policies with the skill prior and decoder, respectively. After 1M steps of HL policy training, we perform the full Skill-Critic Algorithm 2 with the iterative HL and LL policy updates. We found this step was critical for the success of the Skill-Critic algorithm in maze tasks (see Fig. \ref{Fig: warm-start} for comparison with and without SPiRL warm-starting in the Maze navigation task). Warm-starting the policy allowed the HL policy, $\pi_z$, and the HL Q-value function, $Q^z$, to find a solution to the maze prior to LL policy fine-tuning. We found that this stabilizes this \newtextsmall{parallel} optimization of the HL and LL policies once they are updated iteratively by Skill-Critic. Otherwise, if the HL and LL policy are \newtextsmall{optimized in parallel} immediately before the goal state is discovered, the LL policy may deviate too much from the offline skills, and the goal may not be found (red line in Fig. \ref{Fig: warm-start}). We do not apply the SPiRL warm-start to the racing environment in Fig. \ref{fig:RaceResults}, as we found it did not have a major effect.

\paragraph{Architecture and Hyperparameters.} The LL policy architecture is identical to the decoder architecture, and the HL policy architecture is identical to the skill-prior architecture. Both the HL and LL critics consist of a 2-layer MLP with 256 hidden units per layer. We use a batch size of 256 for the network training of both the HL and LL policies. The discount factor is $\gamma=0.99$. We use the Adam optimizer with $\beta=0.99$ and learning rate 3e-4 to take steps on each loss function. Following SAC \cite{haarnoja2018soft}, for both the HL and LL Q-values, two separate critic networks are trained and the Q-value is the minimum of two critics. The target network update rate is $\tau =5e-3$. The output action is squashed to $[-1, 1]$ by the $\tanh$ function. In Algorithm \ref{Alg:skill-critic-summary}, HL and LL updates are done iteratively, i.e. the loss is calculated and a gradient step is taken on the HL update, then the LL update, then the HL update, and so on. Between each rollout, the total number of steps taken on for each HL and LL update is 200 and 64 for the maze and racing environments, respectively. 

Additional hyperparameters for maze and racing environments are listed in Table~\ref{tab:RL hyperparamter}. The variance of the action prior in the racing environment is different depending on the action, namely $-4.5$ for the steering dimension and $-3.5$ for the throttle dimension. Following \cite{haarnoja2018soft, pertsch2021accelerating, pertsch2021guided}, we use automatic tuning of $\alpha_z$ and $\alpha_a$ with corresponding target divergences $\delta_z$ and $\delta_a$.  $N^\mathcal{H}$ and $N^\mathcal{L}$ steps are taken on the HL and LL update as shown in Algorithm \ref{Alg:skill-critic-summary}. The HL update and LL update retain their own replay buffers; during Skill-Critic, these are filled with the same rollouts as shown in Algorithm \ref{Alg:skill-critic-summary}. 

At the beginning of Skill-Critic training, we sample rollouts with the initial, untrained policy to partially fill the replay buffers. For the only Maze environments, we likewise fill the replay buffer for the SPiRL warm-start. The initial rollout steps for each replay buffer are shown in Table~\ref{tab:RL hyperparamter}.
% \textcolor{red}{In SPiRL and Skill-Critic experiments, we initially sample rollouts with initial steps in Table~\ref{tab:RL hyperparamter} to fill in the replay buffers. }

% In the Maze tasks, the HL policy is warm-started by SPiRL. Before this step, the replay buffer is initialized with the initial steps in Table \ref{tab:RL hyperparamter} using the skill prior, $p_{\psi_z}(z|s)$ as the HL policy and the decoder $g_{\psi_a}(a|s,z)$; this step is also performed by SPiRL \cite{pertsch2021accelerating}. After SPiRL runs for 1M steps, the Skill-Critic replay buffer is filled with initial steps from the SPiRL policies. Then Skill-Critic training begins. For the autonomous racing task, SPiRL warm-start is not performed, and the Skill-Critic replay buffer is initialized using the skill prior, $p_{\psi_z}(z|s)$, as the HL policy and the decoder $g_{\psi_a}(a|s,z)$ as the LL policy.

\begin{table}[b]
    \centering
    \caption{Hyperparameters in downstream RL}
    \label{tab:RL hyperparamter}
\begin{tabular}{lcccc}
\hline \hline
                          & \multicolumn{2}{c}{\textbf{Maze}} & \multicolumn{2}{c}{\textbf{Racing}} \\
                         Policy update & HL on $M^\mathcal{H}$       & LL on $M^\mathcal{L}$          & HL on $M^\mathcal{H}$            & LL on $M^\mathcal{L}$           \\ \hline          \vspace{6pt}
                         Action-prior variance & n/a      &  $\log \sigma_{\hat{a}}= \begin{bmatrix}-3\\-3
         \end{bmatrix}$       & n/a           & $\log \sigma_{\hat{a}}=\begin{bmatrix}-4.5\\-3.5
         \end{bmatrix}$        \\

                         Target KL divergence     & $\delta_z=1$          & $\delta_a=80$          & $\delta_z=5$            &$\delta_a=80$           \\ 
                         % Gradient steps per update & $N^\mathcal{H}=200$ & $N^\mathcal{L}=200$ & $N^\mathcal{H}=64$ & $N^\mathcal{L}=64$ \\
Replay buffer size       & 1e5        & 5e5       & 1e6          & 1e6        \\
% SPiRL buffer initial steps & 5e3        & 5e4       & n/a     & n/a    \\    
Replay buffer initial steps & 5e3        & 5e4       & 4.8e3       & 4.8e4  \\

\hline \hline
\end{tabular}
\end{table}

% \begin{table}[th]
%     \centering
%     \caption{Hyperparameters in downstream RL}
%     \label{tab:RL hyperparamter}
% \begin{tabular}{lcccc}
% \hline \hline
%                          & \multicolumn{2}{c}{Maze} & \multicolumn{2}{c}{Racing} \\
%                          & HL          & LL         & HL           & LL          \\ \hline
% Replay buffer size       & 1e-5        & 5e-5       & 1e-6          & 1e-6        \\
% Warm-start steps         & 5e3        & 5e4       & 4.8e3       & 4.8e4            \\
% Initial variance(logstd) & -      &  [-3, -3]       & -           & [-4.5, -3.5]        \\
% Target KL divergence     & 1          & 80          & 5            &80           \\ 
% Update time per episode & 200 & 200 & 64 & 64 \\
% \hline \hline
% \end{tabular}
% \end{table}

% ================================

\section{Environment and Data Collection}\label{Appendix: env}
We run the experiments with 3 random seeds and present the average and standard deviation across seeds in all results.

\textbf{Maze Demonstrations.}
The maze navigation environment utilized in this study is based on the point maze environment from the D4RL framework~\cite{fu2020d4rl}. To generate the training data, we use the exact demonstrations from SPiRL~\cite{pertsch2021accelerating}. These demonstrations consist of randomly generated, simple maze layouts consisting of walls and doorways placed at random positions. The start and goal positions are randomly positioned within the empty spaces of the maze. The RL agent perceives the environment through an agent-centric top-down view with dimensions of $32\times32\times3$ pixels. For the image-based state inputs, we first pass the state through a convolutional encoder network with three layers, and a kernel size of three (8, 16, 32) channels, respectively. Additionally, to capture the agent's velocity, we incorporate two consecutive observations as input (this is also done in SPiRL). The RL agent's actions are represented as two-dimensional vectors, indicating the velocity in the horizontal and vertical directions. The demonstrations are collected using the D4RL planner that uses tabular Q-learning with actions limited to four directions: up, down, left, and right. Consequently, the learned skills cannot effectively handle diagonal movements or execute smooth curves.

\textbf{Maze Navigation Task. }
We manually design the target maze navigation environment using the D4RL simulator, and it is different than the manual maze environment employed by SPiRL \cite{pertsch2021accelerating}. In this environment, the agent starts at the bottom left corner and must navigate through a series of tunnels at each intersection to reach the goal point located at the top center. The width of both horizontal and vertical tunnels is 1 unit. Additionally, the maze has \textit{diagonal} tunnels that are composed of $1\times1$ empty spaces. The agent is rewarded when its distance to the goal point is less than 1 unit, and it can continue earning rewards until the end of the episode, with a maximum number of steps of 2000.

\textbf{Maze Trajectory Planning Task.}
We likewise manually design the maze trajectory planning task using the D4RL simulator. There is a curvy tunnel with a width of 2 units that extends from the start to the goal point. The agent has more choices to plan trajectories with higher velocity and fewer steps, and can obtain greater rewards. In the D4RL environment, the agent is discouraged from wall contact because the velocity perpendicular to the wall is set to zero whenever the agent is in contact with the wall.  It is important to note that the actions (velocities) and acceleration of the agent are limited, which means that the time-optimal trajectory may not necessarily be the minimum distance path. The ultimate objective in this environment is to plan time-optimal trajectories, namely trajectories that require the least time steps to reach the goal.

\textbf{Autonomous Racing.}
For the autonomous racing experiment, we conduct the data collection and experiments in the Gran Turismo Sport (GTS) high-fidelity racing simulation game. GTS provides highly complex vehicle dynamics models and boasts a large player base$^2$\footnote{$^2$For more information, visit \url{http://www.kudosprime.com}}, and has previously been used to test RL algorithms \cite{fuchs2021super, wurman2022outracing}. In our experiments, we control the \textit{Audi TT Cup '16} car on the \textit{Tokyo Expressway Central Outer Loop} track. The track is bounded by walls, and collisions with the walls result in a reduction of the car's velocity. Our observations, consistent with \cite{fuchs2021super}, include the car's velocity, acceleration, future centerline curvature, and Lidar distance to the wall edge. The actions taken by the agent are the steering wheel angle and the combined throttle/brake pedal command. The agent can observe states and send actions to the environment at a frequency of 10 Hz. The agent selects actions between [-1, 1]. For the steering command, the agent's action is then scaled to the max steering value of $30^\circ$. For the throttle/brake command, if the agent's action is positive, the agent's action is the throttle opening fraction from 0 to 1. Otherwise, if the agent's action is negative, the agent's action is the brake pedal fraction from 0 to 1. See \cite{fuchs2021super} for more details about the GTS environment and its interface. 

Unlike \cite{fuchs2021super}, our autonomous racing tasks focus on a \emph{sparse reward} that is gained only after the car has traveled sufficiently far on the track. Specifically, only a corner of the racetrack (1200 meters long) is used, depicted in Fig.~\ref{fig:env_racing}. 
To collect offline demonstrations, we utilize the built-in AI agent in GTS, which employs a rule-based controller to follow a predefined low-speed trajectory on the track. Specifically, the agent is initialized at the course centerline with a low velocity (10 m/s); its progress along the track is randomly initialized within the corner. Its initial pose is parallel to the heading of the centerline. We create 40000 demonstration trajectories, each 200 steps in length. During the downstream racing task, the agent has episode lengths of 600 steps (60 seconds) and will receive a reward of +1 for as long as it is \textit{after} the goal point on the track. It is initialized before the corner as shown in Fig. \ref{fig:env_racing} at a low speed (10 m/s) with a heading parallel to the centerline of the track. Thus, to finish the corner in the least amount of time, the agent must learn to speed up when entering the corner, slow down and navigate the corner, and then speed up when exiting the corner.
